# Supplementary material for: Parametric Lattices Are Better Quantizers in Dimensions 13 and 14
Source: arXiv:2411.19250 ancillary file (2024-11-28)
Supplement: Supplementary file 1 [file anc_f2f3.pdf]

EXPRESSIONS FOR  $f_2^B$  AND  $f_3^B$

This supplementary material for the manuscript *Parametric Lattices Are Better Quantizers in Dimensions 13 and 14* by Daniel Pook-Kolb, Erik Agrell, and Bruce Allen contains the full expressions for the functions  $f_2^B$  and  $f_3^B$  defined in Eq. (66). They are

$$\begin{aligned} f_2^B(v_2, v_3) &= \frac{\sum_{i=0}^{14} \sum_{j=0}^{14-i} c'_{i,j} v_2^i v_3^j}{2^{79} \cdot 3^{10} \cdot 5^3 \cdot 7^3 \cdot 11^2 \cdot 13^4}, \\ f_3^B(v_2, v_3) &= \frac{\sum_{i=0}^{14} \sum_{j=0}^{14-i} c''_{i,j} v_2^i v_3^j}{2^{77} \cdot 3^{10} \cdot 5^4 \cdot 7^3 \cdot 11^2 \cdot 13^4}, \end{aligned} \tag{1}$$

where the integer coefficients  $c'_{i,j}$  and  $c''_{i,j}$  are given in Tab. I and Tab. II, respectively.

TABLE I  
COEFFICIENTS  $c'_{i,j}$  OF  $f_2^B(v_2, v_3)$  IN (1).

| $i$ | $j$ | $c'_{i,j}$                               | $i$ | $j$ | $c'_{i,j}$                                 |
|-----|-----|------------------------------------------|-----|-----|--------------------------------------------|
| 0   | 0   | -251640026909471328252292085946777600    | 4   | 6   | -276514353497465287946864944868889722880   |
| 0   | 1   | 168655185338680620078114161477812224     | 4   | 7   | -73398793391801463323782743455139102720    |
| 0   | 2   | -7520372646873393260552113243000143872   | 4   | 8   | -26357569379376661446945130701993738240    |
| 0   | 3   | 13132781497370971457109759343206596608   | 4   | 9   | -8934325984032511157082532258503229440     |
| 0   | 4   | -24051590640089013135912901144210309120  | 4   | 10  | -1846517845009485925558170951266709504     |
| 0   | 5   | 17902245769661577516234971839541542912   | 5   | 0   | 34956051772121658449070421588270120960     |
| 0   | 6   | -21700268050905587157859488859638398976  | 5   | 1   | 24989937539583790710362066434004090880     |
| 0   | 7   | 14789506183604496568190238090382147584   | 5   | 2   | 328154858489400876108862346084336271360    |
| 0   | 8   | -18843382993156068426632990159000678400  | 5   | 3   | 513578029119702555523517451094626140160    |
| 0   | 9   | 16017998605040893123596038826017769472   | 5   | 4   | 416447175178762699904398693494769582080    |
| 0   | 10  | -11292517590464066619249640891215169792  | 5   | 5   | 219221670755454725504564550539170283520    |
| 0   | 11  | 5342476954773569137362529630506588928    | 5   | 6   | 85048353764579098111547131284412170240     |
| 0   | 12  | -1751361615275740791966271400297205680   | 5   | 7   | 22881560219275258314923432137237463040     |
| 0   | 13  | 320865207446946254611184439814107704     | 5   | 8   | 7366358847287340513567163219985694720      |
| 0   | 14  | -32595890173718460204133986503458017     | 5   | 9   | 1434247692563865747496869971471400960      |
| 1   | 0   | 1561246888553478504434604323421290496    | 6   | 0   | 125918488606486747064509344100254744576    |
| 1   | 1   | -6434998677038371871286977817439371264   | 6   | 1   | 759408598602310109372968817099878170624    |
| 1   | 2   | 45936665157126865549664818119045021696   | 6   | 2   | 1048083008575174219824877335319928635392   |
| 1   | 3   | -55227203459720614087264476314550140928  | 6   | 3   | 1176723334552734315794052651963396390912   |
| 1   | 4   | 153801990051654884156544197853802659840  | 6   | 4   | 782088234601789969765182789780001259520    |
| 1   | 5   | -75844490233071760634681879889018617856  | 6   | 5   | 346329358082871339548060285867831328768    |
| 1   | 6   | 109161807836790675201558616482727329792  | 6   | 6   | 104674316866890409530589806482562220032    |
| 1   | 7   | -8768564501809222145217461330102059008   | 6   | 7   | 27308156460130525603284856527227191296     |
| 1   | 8   | 3089912960646448803083922825937969152    | 6   | 8   | 5149044904850237503474994618399981568      |
| 1   | 9   | 12775734144198074979086846118991841280   | 7   | 0   | -556433822489461487770451424850181357568   |
| 1   | 10  | -6311263791273664747743774424360178688   | 7   | 1   | -2261726363799242196412959876301556023296  |
| 1   | 11  | 2939687385673857983993610838692470016    | 7   | 2   | -3436585002198811335310123084262211059712  |
| 1   | 12  | -361495565501449924347539936965120992    | 7   | 3   | -3159843543473116383144759196526460272640  |
| 1   | 13  | 91454679813578099672994571598381784      | 7   | 4   | -1688640088292095594657659840995115663360  |
| 2   | 0   | -5443640639134211801834911186263474176   | 7   | 5   | -58852414326893072324056583330765856768    |
| 2   | 1   | -5258295144624516703574483243762712576   | 7   | 6   | -144139487449506275140567989764807983104   |
| 2   | 2   | -131552522751456351144163800839601782784 | 7   | 7   | -24559847326551987548032800497174839296    |
| 2   | 3   | -1331155038046297792645264829778493440   | 8   | 0   | 114604327867299608656369684061243556593664 |
| 2   | 4   | -388200921914793108610474709876861829120 | 8   | 1   | 3855386041798928855096219868943494414336   |
| 2   | 5   | -985796734864212288273777315299721216    | 8   | 2   | 5018838607334280950228951770685169991680   |
| 2   | 6   | -260762320293132971212324591955708215296 | 8   | 3   | 3659309019855332165640239116409980846080   |
| 2   | 7   | 9569039917105017761191312633648644096    | 8   | 4   | 1512675994602946276745664809699660267520   |
| 2   | 8   | -41694190523189740872140963804897771520  | 8   | 5   | 392091045860582300175074616289416708096    |
| 2   | 9   | 601289436992298126386402302086512640     | 8   | 6   | 6097333170123445447272035917556350976      |
| 2   | 10  | -3763028721757972168854090417725190144   | 9   | 0   | -1523337410877658160933707461243556593664  |
| 2   | 11  | -953673153297594710224729692335192064    | 9   | 1   | -4184894954702201438499074921030368624640  |
| 2   | 12  | -257687276401454061351534001339050368    | 9   | 2   | -4435163367685903227393393795828379811840  |
| 3   | 0   | 17617572408885953564950054463011291136   | 9   | 3   | -2441381124703118604162989296597294120960  |
| 3   | 1   | 70658111939501664507917375044159799296   | 9   | 4   | -719448985092280730353791989142268149760   |
| 3   | 2   | 323776038967734016691808189836657950720  | 9   | 5   | -110368707933554082735065694239188844544   |
| 3   | 3   | 347967765303378192805916280497708728320  | 10  | 0   | 1396391152999150610994760162679287971840   |
| 3   | 4   | 741626757500322477639941636741042012160  | 10  | 1   | 3038693558818334780047849236887324590080   |
| 3   | 5   | 29485655355183168969918222232717361152   | 10  | 2   | 2452196411100849072349848166584822005760   |
| 3   | 6   | 364242110692115202113495143471065858048  | 10  | 3   | 9271873250071324047655585196539046789120   |
| 3   | 7   | 37686001402774672580274738989369917440   | 10  | 4   | 152795610300059818061245945769329950720    |
| 3   | 8   | 45974809396879523572732377828081991680   | 11  | 0   | -885735036973984247164896737663331074048   |
| 3   | 9   | 5794521655566152126412481635013345280    | 11  | 1   | -1442730471477723383138438623938691989504  |
| 3   | 10  | 4831916325683786599296420075217670144    | 11  | 2   | -793026840371501479441371564504709595136   |
| 3   | 11  | 816855992912904209017285241261908992     | 11  | 3   | -159457011817883429760809957093913133056   |
| 4   | 0   | -41264007596696439951662569580138594304  | 12  | 0   | 374236389168257156366601181625820643328    |
| 4   | 1   | -184165950559320784236243263035161968640 | 12  | 1   | 408884278469505908274137302219270127616    |
| 4   | 2   | -579369860190350741462108816102349864960 | 12  | 2   | 116559573282842146207117313494061416448    |
| 4   | 3   | -772685506579906570177047207119180267520 | 13  | 0   | -95380764936245304885932149446568574976    |
| 4   | 4   | -934831269490484638380679150429557227520 | 13  | 1   | -52986246342959422669743184566703620096    |
| 4   | 5   | -524201044334870666024371046584216977408 | 14  | 0   | 1116312730442023843858889869009813504      |

TABLE II  
COEFFICIENTS  $c''_{i,j}$  OF  $f_3^B(v_2, v_3)$  IN (1).

| $i$ | $j$ | $c''_{i,j}$                               | $i$ | $j$ | $c''_{i,j}$                               |
|-----|-----|-------------------------------------------|-----|-----|-------------------------------------------|
| 0   | 0   | -62910006727367832063073021486694400      | 4   | 6   | 1228952682210956835319399754972843212800  |
| 0   | 1   | 30117056881047868215680610026389504       | 4   | 7   | 392479659108938380273004947642063257600   |
| 0   | 2   | 1611508424330012841546881409214316544     | 4   | 8   | 164734808621104134043407066887460864000   |
| 0   | 3   | -5862848882754897971923999706788659200    | 4   | 9   | 63905248358010322859687557126793932800    |
| 0   | 4   | 16320722220060401770798040062142709760    | 4   | 10  | 14874727084798636622551932662981826560    |
| 0   | 5   | -16303830968798936666571135068153905152   | 5   | 0   | 122346181202425804571746475558945423360   |
| 0   | 6   | 24800306343892099608982272982443884544    | 5   | 1   | 6247484384895947677590516608501022720     |
| 0   | 7   | -20335571002456182781261577374275452928   | 5   | 2   | -984464575468202628326587038253008814080  |
| 0   | 8   | 30284008381857967114231591326965376000    | 5   | 3   | -3209862681998140972021984069341413376000 |
| 0   | 9   | -29461676005700214138042714269282683136   | 5   | 4   | -3956248164198245649091787588200311029760 |
| 0   | 10  | 23391643580246995139874256131802851712    | 5   | 5   | -2795076302132047750183198019374421114880 |
| 0   | 11  | -12306777270817686048567255755988392352   | 5   | 6   | -1360773660233265569784754100550594723840 |
| 0   | 12  | 4440952667306342722485902479325057260     | 5   | 7   | -440470034221048722562276068641821163520  |
| 0   | 13  | -888109056326369097584528360199762395     | 5   | 8   | -165743074063965161555261172449678131200  |
| 0   | 14  | 97787670521155380612401959510374051       | 5   | 9   | -36931878083519542998044401765388574720   |
| 1   | 0   | 479330185082208312765010099296010240      | 6   | 0   | -275446693826689759203614190219307253760  |
| 1   | 1   | -141118392040315172615942495996477440     | 6   | 1   | -118657593531610954589526377671855964160  |
| 1   | 2   | -12088596093980754092017057399748689920   | 6   | 2   | 196515564107845166217164500374866191360   |
| 1   | 3   | 3027807207215248951351138330345472000     | 6   | 3   | 4596575525596618421070518171732017152000  |
| 1   | 4   | -128168325043045736797120164878168883200  | 6   | 4   | 4643648892948127945480772814318757478400  |
| 1   | 5   | 84826074602777627025631049875876085760    | 6   | 5   | 2759812072222880987023605403009280901120  |
| 1   | 6   | -153209554858653579230257707344178708480  | 6   | 6   | 1046743168668904095305898064825622200320  |
| 1   | 7   | 14806567250862063710125976368812687360    | 6   | 7   | 328551257410945386164520930093202145280   |
| 1   | 8   | -6098512422328517374507742419614412800    | 6   | 8   | 72408443974456464892617111821249740800    |
| 1   | 9   | -28857469667815827255393533996845606400   | 7   | 0   | 463694852074551239808709520708484464640   |
| 1   | 10  | 16054969293590901551278022658460103680    | 7   | 1   | 134626569273764416453152373589378334720   |
| 1   | 11  | -8316220893682624559981925398932645440    | 7   | 2   | -2454703572999150953792945060187293614080 |
| 1   | 12  | 1125709875026444939854181382654543440     | 7   | 3   | -4702148130168327951108272613878661120000 |
| 1   | 13  | -310865687962820294941099969248885450     | 7   | 4   | -3819543056851168606963754402250856857600 |
| 2   | 0   | -2165084345110197875729794221809336320    | 7   | 5   | -1786591149209253981266003422611253493760 |
| 2   | 1   | -149383384790469224533366001243258880     | 7   | 6   | -549102809331452476725973294342125649920  |
| 2   | 2   | 44847450937996483344601295740773335040    | 7   | 7   | -112565966913363276261817002278718013440  |
| 2   | 3   | 9454226071055609227731011952967800000     | 8   | 0   | -589875216964042103378373303654515752960  |
| 2   | 4   | 419080540703469833159035198162521292800   | 8   | 1   | -141742133889666502025596318711157882880  |
| 2   | 5   | 1428285041990762122214847814780846080     | 8   | 2   | 2214193503235712183924537545890516172800  |
| 2   | 6   | 474113309623878129476953803555833118720   | 8   | 3   | 3363335496190562652242866834935644160000  |
| 2   | 7   | -20932274818667226352605996386106408960   | 8   | 4   | 2113297345401174945453502307668643020800  |
| 2   | 8   | 106604464405882860184451327910249984000   | 8   | 5   | 735170710988591812828264905542656327680   |
| 2   | 9   | -1759454886653599631187484008946329600    | 8   | 6   | 143466662826434010527698908041309061120   |
| 2   | 10  | 12400890105793317374632797967503467520    | 9   | 0   | 567200099794872719496593203654515752960   |
| 2   | 11  | 3494995362937207886903128702023857280     | 9   | 1   | 111300397731441527619656247899743846400   |
| 2   | 12  | 1039533899119502179315847391765487280     | 9   | 2   | -1415477670538054221508529934838844620800 |
| 3   | 0   | 9945403779209812496342772680732180480     | 9   | 3   | -1623258726531328859150923734439690240000 |
| 3   | 1   | 2849117416915389697899894155006443520     | 9   | 4   | -727102697699645418974577010303356108800  |
| 3   | 2   | -156665825306968072592810414437092556800  | 9   | 5   | -149702236824767505837456127824431677440  |
| 3   | 3   | -350773956959050597586609153727528960000  | 10  | 0   | -407280752958085594873471714114792325120  |
| 3   | 4   | -1136363580040816699609587991780628889600 | 10  | 1   | -63306115808715307917663525768485928960   |
| 3   | 5   | -606358235133642807155880215075346186240  | 10  | 2   | 613049102775212268087462041646205501440   |
| 3   | 6   | -939979640495781166744503596054363504640  | 10  | 3   | 482910065107881460815408956530753536000   |
| 3   | 7   | -117008955968292330188756246055704985600  | 10  | 4   | 120963191487547355965153040400719544320   |
| 3   | 8   | -166844066359643432320399758247071744000  | 11  | 0   | 212333741740338689388845108343949230080   |
| 3   | 9   | -24065956875940067299213129371224780800   | 11  | 1   | 24704288895166496286617099724977602560    |
| 3   | 10  | -22600898942714485706386480996985876480   | 11  | 2   | -162950720624281125912610595446173204480  |
| 3   | 11  | -4248968672813090442065717585596220160    | 11  | 3   | -68260707113819961370209741906640896000   |
| 4   | 0   | -40117785163454872175227498202912522240   | 12  | 0   | -76152753609819770190878147423858851840   |
| 4   | 1   | -12789302122175054460850226599664025600   | 12  | 1   | -5943085442870725410961297997373112320    |
| 4   | 2   | 482808216825292284551757346751958220800   | 12  | 2   | 20330158130728281315194880260592107520    |
| 4   | 3   | 1341467893367893351001818067915243520000  | 13  | 0   | 16860236226103968035392046619342929920    |
| 4   | 4   | 2466915850044334462393458869189109350400  | 13  | 1   | 669018261906053316537161421296762880      |
| 4   | 5   | 1856545365352666942169647456652435128320  | 14  | 0   | -1744238641315662256029514042032783360    |
